# Supplementary material for: Fast Search-By-Classification for Large-Scale Databases Using Index-Aware Decision Trees and Random Forests
Source: arXiv:2306.02670 source file (2023-07-31)
Supplement: Supplementary file 1 [file 07_appendix.tex]

% All given parameters \todot{which ones?} can be inserted into the function \texttt{run\_experiment}. An example for the general usage of this function is given in the repository. If not defined in the hyperparameter grid, the default values are used \todot{list default parameters of decision branch / ensemble}.
% \begin{itemize}
%     \item \todot{Christian: more details}
% \end{itemize}

% \subsection{Implementation Details}
% Both \tdecisionbranch model and the \kdtree are majorly implemented in Python. Computational intense sections of the core algorithms make use of Cython for the sake of runtime performance. 
%In contrast to Python, Cython offers C-like performance with the ease of Python code. 
%The computational overhead caused by pure Python code would have impeded the runtime of the whole process. This would contradict with the overarching goal of minimizing the query time for rare object search. 

% \begin{itemize}
%     \item \todot{Christian: We have 2 pages of "supplenmental material" that we can use for explanations regarding the reproducibility and algorithms that do not fit in the main manuscript. Please provide detailed comments regarding the reprodibility; i}
% \end{itemize}
% \section{Implementation Details}
% We provide some further technical details related to our approach as well as information regarding the reproducibility of our results.

% \subsection{Notation}
% \begin{table}[H]%[t]
%     \centering
%     %\vspace{-11pt}
%     \caption{\blue{Summary of notations.}}
%     {
%     \color{blue}
%     \resizebox{1.0\columnwidth}{!}{
%     \begin{tabular}{ll}
%         \toprule
%         Notation     & Description\\
%         \midrule
%         $B$ & Box\\
%         $\decisionbranchmodel$ & Decision branch model\\
%         $c$ & Class identifier\\
%         $c_n$ & Non-rare class\\
%         $c_r$ & Rare class\\
%         $\mathcal{C}(h_1(\vec{x}) \ldots h_M(\vec{x}))$ & Aggregration function of tree ensembles (e.g., majority vote)\\
%         $d$ & Dimensionality of data set\\
%         $D$ & Dimensionality of feature subset\\
%         $\featuresubset$ & Feature subset\\
%         $\mathcal{F}$ & Set of feature subsets\\
%         $\greedygain$ & Gain\\
%         $G(S)$ & Information gain function\\
%         $\predfunc(\vec{x})$ & Prediction function\\
%         $\dtboxdimupperbound$ & Upper bound for features of box\\
%         %$i$ & Splitting dimension \todot{Overloaded variable!!! splitting dimension and identifier} \\
%         $O$ & Subset of points not contained in $B$ where $O \subseteq S$ and $O= S\backslash I$\\
%         $I$ & Subset of points contained in $B$ where $I \subseteq S$\\
%         $\tsizesubsets$ & Number of feature subsets\\
%         $\nclasses$ & Number of classes\\
%         $l$ & Left bound of box\\
%         $\tsize$ & Size of training set\\
%         $\dtnumberbounded(B)$ & Number of bounded dimensions for box $B$\\
%         $\dtnumberunbounded(B)$ & Number of unbounded dimensions for box $B$\\
%         $\testsize$ & Size of test set\\
%         $m$ & Model identifier\\
%         $\forestNTrees$ & Number of models in ensemble\\
%         $\numberfeaturesubsetstest$  & Number of feature subsets tested in one iteration\\
%         $\greedymaxpoints$ & Number of points tested in one iteration\\
%         $p_S^c$ & Fraction of points in $S$ of class $c$\\
%         $\precision$ & Precision\\
%         $\indexStructuresQueryPoints$ & Number of points returned by query\\
%         $Q(S)$ & Impurity measure\\
%         $r$ & Right bound of box\\
%         $R$ & Set of training points to be removed \\
%         $\recall$ & Recall\\
%         $S$ & Subset of $T$ ($S \subseteq \trainset$) \\
%         $\trainset$ & Training set\\
%         $\mathcal{T}$ & Model instance\\
%         \querytime & Query time\\
%         \totaltime & Total time \\
%         \trainingtime & Training time\\
%         $\vec{x}$ & Feature vector\\
%         $x$ & Feature value\\
%         $y$ & Label  \\
%         $\theta$ & Splitting threshold\\
%         $\mu$ & Number of features per split \\
%         $\multiplicationfactor$ & Multiplication factor\\
%         \bottomrule
%     \end{tabular}
%     }
%     }
% \label{tab:all_db_parameter}
% \end{table}

% \subsection{Recurrent Rare Object Search via Tree-based Classification Models}
% \vskip-0.2cm
% \blue{Unlike other approaches that are based on finding nearest neighbors (see Section 2.3 of the main manuscript), we take into account non-rare objects that can be defined by the user in advance to make the search more precise. We model this search as a highly imbalanced, binary classification task, where the training set includes labeled rare and non-rare objects. That is, we answer recurrent user queries under a \emph{search-by-classification} approach. 
% To illustrate our motivation and contribution, we compare two different methods for searching rare objects in massive data catalogs, which are depicted in Figure~\ref{fig:intro}.
% In traditional scenarios (left figure), one would train a machine learning model and apply it on the extremely large test set. However, this would require to scan the whole data set. \emph{In contrast, our method learns decision boundaries (i.e., hyperboxes) that can be transformed into orthogonal range queries, which are supported by efficient index structures} (right figure). By leveraging such index structures, we significantly decrease the search time and avoid scanning the entire data set. Naturally, this requires the index structures to be pre-built and loaded into memory in advance. Therefore, our approach targets ideally scenarios where multiple (e.g., thousands) searches must be processed over a \emph{extremely large dataset}, which is typically the case for the increasing number of search engines available online. Note that the pre-build index structures are not task-specific, and hold for all upcoming queries (i.e., different search tasks). They therefore have to be built only once for all the incoming user queries.}
% \begin{figure*}[t]
%     \centering
%     \subfigure{
%         \includegraphics[width=0.45\textwidth]{figures/figure1/Figure_1_part1.pdf}
%         \label{fig:intro1}
%     }
%     \hfill
%     \subfigure{
%         \def\svgwidth{0.45\textwidth}
%         \import{figures/figure1}{Figure_1_part2.pdf_tex}	
%         % \includegraphics[width=0.45\textwidth]{figures/figure1/Figure_1_part2.pdf}
%         %\label{fig:intro2}
%     }
%     \caption{\blue{Comparison of two rare-object search methods. \textit{Left:} full scan of the data set based on traditional decision trees. \textit{Right:} index-supported search based on our decision branch models. Only a small fraction of the data needs to be touched. Indexes are used to speed-up the search.}}
%     \label{fig:intro}
%     \vspace{-12pt}    
% \end{figure*}




% \subsection{Implementation Details}
% Both the bottom-up construction scheme for decision branches as well as the hybrid memory version of $k$-d trees (see below) are majorly implemented in Python~3.8, where Cython is used for the computationally intense parts. 
% Next, we provide details related to the function \textsc{InitialEmptyBox} used in Algorithm~\ref{alg:greedy_max_gain_box}, to the hybrid memory scheme for \kdtrees, to different ways of implementing the function \textsc{TopDownConstruct} in Algorithm~\ref{alg:bottom_up_construct}, as well as to the extraction of features for the geospatial case study.



% \subsubsection{Feature Extraction}
% The geospatial case study is based on image patches such as the ones shown in Figure~\ref{fig:classes} in the main manuscript. Decision trees and decision branches as well as the corresponding ensembles work well in case meaningful features are given. For that reason, we make use of ResNet101 deep neural network architecture to extract 50 features.
% %To extract features to be used by \tdecisionbranches in the geospatial search use case (Section~\ref{sec:geospatial_search}), we train a ResNet101. 
% The neural network is trained on 40,000 image patches belonging to the rare and non-rare classes. 
% %Out of the 40,000 rare-object patches above, 80\% are randomly assigned for training of the ResNet101 and 20\% for test. 
% %Based on the labeled data, we train a ResNet101 to extract features to be used by \tdecisionbranches. 
% Instead of training the network from scratch, we make use of a version pre-trained on the ImageNet data set. We replace the final classification layer with two fully connected layers with output sizes 50 and 7 (6 rare classes and 1 non-rare class), respectively. Only these last two layers are trained by using cross-entropy as loss function and by conducting grid search to identify proper hyperparameters. Finally, data augmentation techniques (rotation, flipping, \ldots) are also used to improve the model quality. We use the 50 outputs of the previous-to-last layer as the extracted features.

% \section{Additional Experiments}
% \subsection{Comparison with Boosted Models}
% \blue{
% In analogy to our previous experiments in Section 4.1, we extended on them by evaluating boosted tree models. We selected Gradient Boosting~\cite{gradientboosting} and XGBoost~\cite{xgboost} for that comparison. In Table \ref{tab:boost}, the results are shown which point out that boosted models are not outperforming the prior tree-based models for our specific use case of highly imbalanced data sets with small training sets. }
% \begin{table}[H]%[ht]
% \caption{\blue{Mean test $\fscore$-scores for boosted models on each data set averaged among all classes.}}
% %\vspace{-5pt}
% \centering
% \blue{
% \begin{tabular}{lrr}
% \toprule
% Data Set &    Gradient Boosting &   XGBoost \\
% \midrule
% covtype  & $0.417 \pm 0.03$ & $0.446 \pm 0.03$ \\
% iris     & $0.972 \pm 0.04$ & $0.978 \pm 0.04$ \\
% letter   & $0.689 \pm 0.03$ & $0.710 \pm 0.03$ \\
% mnist    & $0.621 \pm 0.04$ & $0.528 \pm 0.04$ \\
% satimage & $0.747 \pm 0.03$ & $0.757 \pm 0.02$ \\
% senseit  & $0.576 \pm 0.04$ & $0.544 \pm 0.04$ \\
% \midrule
% \textbf{Total}    & $0.670 \pm 0.04$ & $0.660 \pm 0.03$ \\
% \bottomrule
% \end{tabular}
% }
% \label{tab:boost}
% \end{table}


% \subsection{Space Consumption}
% Choosing the optimal number of feature subsets $\tsizesubsets$ for the indexed box search represents a trade-off between required storage capacities and the accuracy of the results. Building additional indexes further improves the result of our decision branch models and ensembles, while increasing storage consumption. Furthermore, since the accuracy of the results tends to increase using more feature subsets, the search returns fewer false positive instances, which also reduces query processing time. However, as we report in Figure~6 of the main manuscript, there is an upper bound for the number of feature subsets at which increasing the number of feature subsets generally brings no additional benefits in terms of accuracy.
% More precisely, as it can be seen in the figure, $\tau = \frac{\tsizesubsets}{\tdim} \approx 1$ seems to be sufficient for the case of $\tdimsubsets=3$. Thus, using $\tsizesubsets \approx \tdim$ feature subsets of cardinality $\tdimsubsets=3$ leads to $\O(\tdimsubsets \testsize \tdim)$ space overhead to store the features in the leaves of the index structures. Since storing the data requires $\O(\testsize \tdim)$ space, only about $\tdimsubsets$ times additional space is used.
% Generally, the optimal number of feature subsets $\tsizesubsets$ is case-specific and relies on the preferred balance between storage capacities and accuracy of the results. For the case study provided in the main manuscript, $\tsizesubsets=300$ feature subsets are considered. In Tables \ref{tab:res_large_50}, \ref{tab:res_large_100}, and \ref{tab:res_large_150}, corresponding results 
% for  $\tsizesubsets = 50$, $\tsizesubsets = 100$, and $\tsizesubsets = 150$, respectively, are shown. In comparison to the original experiments with $\tsizesubsets = 300$, similar $\fscore$-scores are achieved, while using significantly less additional space for the index structures.

% Another alternative to reducing storage consumption would be to lower the numerical precision of the index structures. In our experiments, we create indexes with 64-bit float precision. Here, 32-bit or even 16-bit might also be sufficient. Finally, reducing the space consumption of index structures is an active field of research. Techniques such as leveraging index compression~\cite{Berchtold2000compression} and learned indexes~\cite{Li2020lisa} could also be used to reduce space consumption even further. 


% \begin{table}[H]%[ht]
% \caption{Results on aerial data set with $\tsizesubsets = 50$ requiring 2.17 TB of storage (time in s).}
% \vspace{-5pt}
% \centering
% %\resizebox{0.8\columnwidth}{!}{
% \begin{tabular}{lrrrr}
% \toprule
%  Model &  \trainingtime &  \querytime &  \totaltime & $\fscore$-score \\
% \midrule
% \decisionbranch{[3]}         &          0.307 &       1.556 &       1.863 &    0.800 \\
% \decisionbranch{[T\textsubscript{s},3]}      &          0.310 &       1.445 &       1.756 &    0.801 \\
% \decisionbranch{[T\textsubscript{a},3]}       &          0.335 &      16.618 &      16.953 &    0.818 \\
% \decisiontree        &          0.855 &     1,043.433 &     1,044.288 &       0.829 \\ \midrule
% \dbensemble{[5t,3]}     &          0.529 &       9.760 &      10.288 &    0.895 \\
% \dbensemble{[T\textsubscript{s},5t,3]}  &          0.508 &       8.418 &       8.926 &    0.884 \\
% \dbensemble{[25t,3]}    &          0.891 &      28.607 &      29.497 &    0.915 \\
% \dbensemble{[T\textsubscript{s},25t,3]} &          0.892 &      26.466 &      27.358 &    0.897 \\
% \randomforest &          0.274 &     1,319.688 &     1,319.961 &        0.904 \\
% \extratrees &          0.122 &     1,332.026 &     1,332.148 &        0.950 \\
% \bottomrule
% \end{tabular}
% %}
% \label{tab:res_large_50}
% \end{table}

% \begin{table}[H]%[ht]
% \caption{Results on aerial data set with $\tsizesubsets = 100$  requiring 4.32 TB of storage (time in s).}
% \vspace{-5pt}
% \centering
% %\resizebox{0.8\columnwidth}{!}{
% \begin{tabular}{lrrrr}
% \toprule
%  Model &  \trainingtime &  \querytime &  \totaltime & $\fscore$-score \\
% \midrule
% \decisionbranch{[3]}         &          0.341 &       1.711 &       2.052 &    0.846 \\
% \decisionbranch{[T\textsubscript{s},3]}      &          0.383 &       1.683 &       2.066 &    0.835 \\
% \decisionbranch{[T\textsubscript{a},3]}     &          0.464 &      13.882 &      14.347 &    0.853 \\
% \decisiontree        &          0.855 &     1,043.433 &     1,044.288 &       0.829 \\ \midrule
% \dbensemble{[5t,3]}     &          0.787 &       7.564 &       8.352 &    0.911 \\
% \dbensemble{[T\textsubscript{s},5t,3]}  &          0.783 &       6.999 &       7.781 &    0.902 \\
% \dbensemble{[25t,3]}    &          1.303 &      24.277 &      25.581 &    0.928 \\
% \dbensemble{[T\textsubscript{s},25t,3]} &          1.425 &      19.188 &      20.613 &    0.915 \\
% \randomforest &          0.274 &     1,319.688 &     1,319.961 &        0.904 \\
% \extratrees &          0.122 &     1,332.026 &     1,332.148 &        0.950 \\
% \bottomrule
% \end{tabular}
% %}
% \label{tab:res_large_100}
% \end{table}

% \begin{table}[H]%[ht]
% \caption{Results on aerial data set with $\tsizesubsets = 150$ requiring 6.5 TB of storage (time in s).}
% \vspace{-5pt}
% \centering
% % \resizebox{0.8\columnwidth}{!}{
% \begin{tabular}{lrrrr}
% \toprule
%  Model &  \trainingtime &  \querytime &  \totaltime & $\fscore$-score \\
% \midrule
% \decisionbranch{[3]}         &          0.398 &       1.047 &       1.445 &    0.833 \\
% \decisionbranch{[T\textsubscript{s},3]}      &          0.399 &       1.090 &       1.489 &    0.824 \\
% \decisionbranch{[T\textsubscript{a},3]}       &          0.420 &      14.685 &      15.105 &    0.833 \\
% \decisiontree        &          0.855 &     1,043.433 &     1,044.288 &       0.829 \\ \midrule
% \dbensemble{[5t,3]}     &          0.993 &       5.666 &       6.658 &    0.914 \\
% \dbensemble{[T\textsubscript{s},5t,3]}  &          1.013 &       5.455 &       6.468 &    0.904 \\
% \dbensemble{[25t,3]}   &          1.543 &      22.639 &      24.182 &    0.925 \\
% \dbensemble{[T\textsubscript{s},25t,3]} &          1.573 &      21.212 &      22.785 &    0.916 \\
% \randomforest &          0.274 &     1,319.688 &     1,319.961 &        0.904 \\
% \extratrees &          0.122 &     1,332.026 &     1,332.148 &        0.950 \\
% \bottomrule
% \end{tabular}
% % }
% \label{tab:res_large_150}
% \end{table}

% \input{figures/mainfigure}

% \begin{table}[hbt]
% \caption{Results on Aerial dataset with 1,441,557,000 objects for \tdecisionbranch models with $\tdimsubsets = 6$ and classic counterparts. Time is shown in seconds. Bold numbers indicate the best result}
% \begin{tabular}{lrrrr}
% \toprule
%       Model &  \trainingtime &  \querytime &  \totaltime & $\fscore$-score \\
% \midrule
%         \decisionbranch [\textit{B}] &         \textbf{ 0.448} &       6.516 &       6.964  &    0.834 \\
%      \decisionbranch [\textit{B,T\textsubscript{s}}] &          0.460 &      \textbf{ 5.409} &       \textbf{5.870} &      0.833 \\
%       \decisionbranch [\textit{B,T\textsubscript{a}}] &          0.549 &      26.109 &      26.659  &    \textbf{0.839} \\
%       \decisiontree        &          0.855 &     1,043.433 &     1,044.288 &       0.829 \\ \midrule
%   \dbensemble [\textit{B,5}] &          1.707 &      \textbf{21.490} &      \textbf{23.197} &       0.899 \\
%  \dbensemble [\textit{B,T\textsubscript{s},5}] &          1.826 &      24.856 &      26.682 &    0.889 \\
%   \dbensemble[\textit{B,25}] &          2.760 &     103.864 &     106.624 &     0.914 \\
% \dbensemble [\textit{B,T\textsubscript{s},25}] &          2.675 &      92.026 &      94.701 &      0.908 \\
%           \randomforest &          0.274 &     1,319.688 &     1,319.961 &        0.904 \\
%           \extratrees &          \textbf{0.122} &     1,332.026 &     1,332.148 &        \textbf{0.950} \\
% \bottomrule
% \end{tabular}
% \label{tab:res_large_dim6}
% \end{table}






% \begin{table*}[]
%     \centering
%     \caption{Caption}
%     \resizebox{\textwidth}{!}{%
% \begin{tabular}{lllllllll|llllllllll}
% \toprule
% Model & \multicolumn{2}{c}{\dbb} & \multicolumn{2}{c}{\dbbts} & \multicolumn{2}{c}{\dbbta} & \multicolumn{2}{c}{\decisiontree} & \multicolumn{2}{c}{\esb} & \multicolumn{2}{c}{\esbts} & \multicolumn{2}{c}{\esbta} & \multicolumn{2}{c}{\randomforest} & \multicolumn{2}{c}{\extratrees} \\
% \cmidrule(lr){1-1} \cmidrule(lr){2-3} \cmidrule(lr){4-5} \cmidrule(lr){6-7} \cmidrule(lr){8-9} \cmidrule(lr){10-11} \cmidrule(lr){12-13} \cmidrule(lr){14-15} \cmidrule(lr){16-17} \cmidrule(lr){18-19}
%  Dataset &   Train & Test &       Train & Test &       Train & Test & Train & Test & Train & Test &     Train & Test &     Train & Test & Train & Test & Train & Test \\
% \midrule
% covtype  &      0.738 &   0.339 &          1.000 &   0.339 &          1.000 &   0.355 &    0.839 &   0.420 &    0.859 &   0.425 &        1.000 &   0.416 &        0.998 &   0.428 &    0.998 &   0.431 &    1.000 &   0.449 \\
% iris     &      0.982 &   0.967 &          1.000 &   0.967 &          1.000 &   0.972 &    0.951 &   0.947 &    0.982 &   0.979 &        0.998 &   0.972 &        1.000 &   0.972 &    0.998 &   0.967 &    1.000 &   0.977 \\
% letter   &      0.901 &   0.525 &          1.000 &   0.578 &          1.000 &   0.585 &    0.938 &   0.580 &    0.986 &   0.721 &        1.000 &   0.749 &        1.000 &   0.759 &    1.000 &   0.677 &    1.000 &   0.735 \\
% mnist    &      0.875 &   0.447 &          0.989 &   0.477 &          1.000 &   0.515 &    0.931 &   0.525 &    0.995 &   0.721 &        1.000 &   0.710 &        1.000 &   0.725 &    1.000 &   0.612 &    1.000 &   0.669 \\
% satimage &      0.940 &   0.659 &          1.000 &   0.669 &          1.000 &   0.675 &    0.902 &   0.653 &    0.971 &   0.742 &        0.999 &   0.773 &        1.000 &   0.767 &    1.000 &   0.755 &    1.000 &   0.781 \\
% senseit  &      0.846 &   0.488 &          1.000 &   0.485 &          0.998 &   0.481 &    0.840 &   0.512 &    0.836 &   0.509 &        1.000 &   0.591 &        1.000 &   0.571 &    0.996 &   0.586 &    1.000 &   0.614 \\
% \bottomrule
% \end{tabular}
% }
% \label{tab:my_label}
% \end{table*}

% \begin{table*}[]
%     \centering
%     \caption{\red{describe that Train and Test stands for F1 score}}
%     \label{tab:my_label}
%     \resizebox{\textwidth}{!}{%
% \begin{tabular}{lllllllllll|llllllllllll}
% \toprule
% Model & \multicolumn{2}{c}{\dbb} & \multicolumn{2}{c}{\dbbts} & \multicolumn{2}{c}{\dbbta} & \multicolumn{2}{c}{\decisiontree} & \multicolumn{2}{c}{\decisiontree[\textit{lim}]} & \multicolumn{2}{c}{\esb} & \multicolumn{2}{c}{\esbts} & \multicolumn{2}{c}{\esbta} & \multicolumn{2}{c}{\randomforest} & \multicolumn{2}{c}{RForest[\textit{lim}]} & \multicolumn{2}{c}{\extratrees} \\
% \cmidrule(lr){1-1} \cmidrule(lr){2-3} \cmidrule(lr){4-5} \cmidrule(lr){6-7} \cmidrule(lr){8-9} \cmidrule(lr){10-11} \cmidrule(lr){12-13} \cmidrule(lr){14-15} \cmidrule(lr){16-17} \cmidrule(lr){18-19} \cmidrule(lr){20-21} \cmidrule(lr){22-23}
% Dataset &   Train & Test &       Train & Test &       Train & Test & Train & Test &  Train & Test & Train & Test &     Train & Test &     Train & Test & Train & Test &    Train & Test & Train & Test \\
% \midrule
% covtype  &      0.738 &   0.339 &          1.000 &   0.339 &          1.000 &   0.355 &    0.839 &   0.420 &     0.464 &   0.217 &    0.859 &   0.425 &        1.000 &   0.416 &        0.998 &   0.428 &    0.998 &   0.431 &       0.995 &   0.157 &    1.000 &   0.449 \\
% iris     &      0.982 &   0.967 &          1.000 &   0.967 &          1.000 &   0.972 &    0.951 &   0.947 &     0.951 &   0.947 &    0.982 &   0.979 &        0.998 &   0.972 &        1.000 &   0.972 &    0.998 &   0.967 &       1.000 &   0.972 &    1.000 &   0.977 \\
% letter   &      0.901 &   0.525 &          1.000 &   0.578 &          1.000 &   0.585 &    0.938 &   0.580 &     0.944 &   0.462 &    0.986 &   0.721 &        1.000 &   0.749 &        1.000 &   0.759 &    1.000 &   0.677 &       1.000 &   0.701 &    1.000 &   0.735 \\
% mnist    &      0.875 &   0.447 &          0.989 &   0.477 &          1.000 &   0.515 &    0.931 &   0.525 &     0.579 &   0.134 &    0.995 &   0.721 &        1.000 &   0.710 &        1.000 &   0.725 &    1.000 &   0.612 &       0.996 &   0.068 &    1.000 &   0.669 \\
% satimage &      0.940 &   0.659 &          1.000 &   0.669 &          1.000 &   0.675 &    0.902 &   0.653 &     0.893 &   0.660 &    0.971 &   0.742 &        0.999 &   0.773 &        1.000 &   0.767 &    1.000 &   0.755 &       1.000 &   0.778 &    1.000 &   0.781 \\
% senseit  &      0.846 &   0.488 &          1.000 &   0.485 &          0.998 &   0.481 &    0.840 &   0.512 &     0.740 &   0.439 &    0.836 &   0.509 &        1.000 &   0.591 &        1.000 &   0.571 &    0.996 &   0.586 &       1.000 &   0.570 &    1.000 &   0.614 \\ \midrule
% \textbf{Total}    &      0.880 &   0.571 &          0.998 &   0.586 &          1.000 &   0.597 &    0.900 &   0.606 &     0.762 &   0.477 &    0.938 &   0.683 &        1.000 &   0.702 &        1.000 &   0.704 &    0.999 &   0.671 &       0.999 &   0.541 &    1.000 &   0.704 \\
% \bottomrule
% \end{tabular}
% }
% \end{table*}





% \begin{table*}[]
%     \centering
%         \caption{Caption}
%     \label{tab:my_label}
% \resizebox{\textwidth}{!}{%
% \begin{tabular}{lccccccccccc}
% \toprule
% & \multicolumn{5}{c}{Single Models} & \multicolumn{6}{c}{Ensemble Models}\\ \cmidrule(lr){2-6} \cmidrule(lr){7-12} 
%  Dataset &  \dbb &  \dbbts &  \dbbta &  DTree &  DTree[lim] &  \esb &  \esbts &  \esbta &  RForest &  RForest[lim] &  ExTrees \\
% \midrule
% covtype  &       $0.339 \pm .033$ & $0.339 \pm .040$ & $0.355 \pm .030$ &  $0.420 \pm .023$ &      $0.217 \pm .121$ &     $0.425 \pm .029$ &  $0.416 \pm .029$ & $0.428 \pm .031$ &    $0.431 \pm .027$ &       $0.157 \pm .025$ &    $0.449 \pm .043$ \\
% iris     &       $0.967 \pm 0.044$ &    $0.967 \pm .044$ &  $0.972 \pm .036$ &  $0.947 \pm .052$ &      $0.947 \pm .052$ &     $0.979 \pm .027$ &         $0.972 \pm .038$ &         $0.972 \pm .038$ &    $0.967 \pm .027$  &      $0.972 \pm .038$ &    $0.977 \pm .029$ \\
% letter   &       $0.525 \pm 0.053$ &           $0.578 \pm .053$ &           $0.585 \pm .049$ &  $0.580 \pm .051$ &      $0.462 \pm .062$ &     $0.721 \pm .036$ &        $0.749 \pm .027$ &         $0.759 \pm .027$ &    $0.677 \pm .054$ &        $0.701 \pm .031$ &    $0.735 \pm .028$ \\
% mnist    &       $0.447 \pm .062$ &           $0.477 \pm .051$ &           $0.515 \pm .047$ &  $0.525 \pm .057$ &      $0.134 \pm .091$ &     $0.721 \pm .036$ &         $0.710 \pm .027$ &         $0.725 \pm .028$ &    $0.612 \pm .068$ &        $0.068 \pm .037$ &    $0.669 \pm .032$ \\
% satimage &       $0.659 \pm .040$ &     $0.669 \pm .046$ &           $0.675 \pm .057$ &  0.653 &      0.660 &     0.742 &         0.773 &         0.767 &    0.755 &        0.778 &    0.781 \\
% senseit  &       $0.488 \pm .056$ &           0.485 &           0.481 &  0.512 &      0.439 &     0.509 &         0.591 &         0.571 &    0.586 &        0.570 &    0.614 \\ \hline
% \textbf{Total}    &       $0.571 \pm .048$ &           0.586 &           0.597 &  0.606 &      0.477 &     0.683 &         0.702 &         0.704 &    0.671 &        0.541 &    0.704 \\
% \bottomrule
% \end{tabular}
% }

% \end{table*}

% \begin{table*}[]
%     \centering
%         \caption{Caption}
%     \label{tab:my_label}
% %\resizebox{\textwidth}{!}{%
% \begin{tabular}{lccccccccccc}
% \toprule
% & \multicolumn{5}{c}{Single Models} & \multicolumn{6}{c}{Ensemble Models}\\ \cmidrule(lr){2-6} \cmidrule(lr){7-12} 
%  Dataset &  \dbb &  \dbbts &  \dbbta &  DTree &  DTree[lim] &  \esb &  \esbts &  \esbta &  RForest &  RForest[lim] &  ExTrees \\
% \midrule
% covtype  &       $0.339$ &           0.339 &           0.355 &  0.420 &      0.217 &     0.425 &         0.416 &         0.428 &    0.431 &        0.157 &    0.449 \\
% iris     &       $0.967$ &           0.967 &           0.972 &  0.947 &      0.947 &     0.979 &         0.972 &         0.972 &    0.967 &        0.972 &    0.977 \\
% letter   &       $0.525$ &           0.578 &           0.585 &  0.580 &      0.462 &     0.721 &         0.749 &         0.759 &    0.677 &        0.701 &    0.735 \\
% mnist    &       $0.447$ &           0.477 &           0.515 &  0.525 &      0.134 &     0.721 &         0.710 &         0.725 &    0.612 &        0.068 &    0.669 \\
% satimage &       $0.659$ &           0.669 &           0.675 &  0.653 &      0.660 &     0.742 &         0.773 &         0.767 &    0.755 &        0.778 &    0.781 \\
% senseit  &       $0.488$ &           0.485 &           0.481 &  0.512 &      0.439 &     0.509 &         0.591 &         0.571 &    0.586 &        0.570 &    0.614 \\ \hline
% \textbf{Total}    &       $0.571$ &           0.586 &           0.597 &  0.606 &      0.477 &     0.683 &         0.702 &         0.704 &    0.671 &        0.541 &    0.704 \\
% \bottomrule
% \end{tabular}
% %}

% \end{table*}
